# Supplementary material for: Contextual Vision Transformers for Robust Representation Learning
Source: arXiv:2305.19402 source file (2023-09-28)
Supplement: Supplementary file 1 [file related.tex]

\section{Related Work}
Our work shares some ideas and expands on the notion of in-context learning proposed in~\cite{brown2020language} in that we realize that a form of conditioning can position transformer-based models to perform test-time adaptation to new tasks, but instead of conditioning on a dataset explicitly for each query infer context tokens which are shareable across a group. 
Similar to~\cite{xie2022explanation} we interpret in-context learning via an implicit generative model, with the key difference that we focus on the case of adaptation to covariate shift and expand that framework with explicit context tokens.
Another related recent work builds hierarchical models for transformers applied to language modeling in~\cite{white2022mixedeffects}, with similar explaining away of group-specific effects and links to mixed models. Our work differs in the implementation details of this idea from the inference strategy of the context tokens to the application to representation learning to images.
Similar to~\cite{hao2022structured}, our approach also achieves test time adaptation without the enormous memory costs of in-context learning since we share inference over the context token across examples using it and only require a single additional token to represent the group information. Test-time adaptation is also the topic of a wealth of prior work~\cite{sun2020test,liu2021ttt++,zhang2022memo}, while on the fly batch norm statistics have been shown to improve CNN generalization at at test time~\cite{zhang2021adaptive,nado2020evaluating, li2016revisiting, schneider2020improving,lin2022incorporating,kaku2020like}. Instead of directly normalizing the feature statistics, our approach abstracts the context information as an extra latent input to the Transformer layer.
Our work also demonstrates value in self-supervised representation learning tasks for ViTs~\cite{zhouimage,he2022masked,assran2022masked,oquab2023dinov2,caron2021emerging}, yielding robustness to covariate shift through context-conditioning during pre-training.

We also would like to highlight the distinction between previous work on prefix tuning~\cite{li2021prefix} and ContextViT. While both approaches involve conditioning a Transformer model with additional tokens, their objectives and mechanisms differ. Prefix tuning focuses on learning a prefix token for a frozen Transformer model, which can enhance performance for a specific downstream task. In contrast, ContextViT aims to generate in-context feature representations by inferring these tokens directly from the input data. Furthermore, ContextViT jointly learns the Transformer parameters along with the context conditioning, as discussed in Section~\ref{sec:cpjump} and Section~\ref{sec:camelyon}.
